# Supplementary material for: Unsupervised Learning for Human Sensing Using Radio Signals
Source: arXiv:2207.02370 source file (2022-07-06)
Supplement: Supplementary file 1 [file appendix.tex]

\section*{Appendix A: Additional Results}
In this section, we provide additional results to better understand the good practices for applying \name~to RGB and RF data.

\textbf{Comparison of Different Reconstructive Tasks for \name's Reconstructive Branch}: In \name, we choose the inpainting task for the reconstructive branch. However, other reconstructive tasks can be potentially used for the reconstructive branch. In this section, we evaluate the performance of \name~with different reconstructive tasks including inpainting, auto-encoder, colorization \cite{zhang2016colorful}, and Jigsaw Puzzle \cite{noroozi2016unsupervised}. Table \ref{tab:ablation} shows \name's performance using different reconstructive task on Colorful-MNIST and RF-based 3D pose estimation (RF-MMD) under the fixed feature extractor setting. As shown in the table, all reconstructive tasks significantly reduce errors in comparison to using contrastive learning without any reconstruction task.  The table also shows that inpaintaing compares favorably to other tasks and works across modalities. Hence, we use inpainting as the default reconstructive task  in \name. 

\begin{table}[h]
\centering
\caption{Comparison of different reconstructive tasks for RCL's reconstructive branch. The table shows 
the performance of \name~on Colorful-MNIST and RF-MMD with different reconstructive tasks in its reconstructive branch for the fixed feature encoder setting. Colorization and Jigsaw Puzzle are not applicable to RF signals. Inpainting achieves the best performance and is applicability across modalities and tasks.}
\label{tab:ablation}
\begin{tabular}{l |@{\hspace{0.2cm}} c c @{\hspace{0.2cm}} |  c @{\hspace{0.2cm}}c  @{\hspace{0.2cm}}c}\toprule[1.5pt]

  & \multicolumn{2}{c|}{Colorful-MNIST}  &  RF-MMD \\
\midrule
Recon. Tasks & \begin{tabular}[c]{@{}c@{}}\textsc{Digit cls} \\ \textsc{Acc.} (\%) \end{tabular} & \begin{tabular}[c]{@{}c@{}}\textsc{Bkgd cls} \\ \textsc{Acc.} (\%) \end{tabular} & Pose \textsc{Err}.$^\downarrow$ (mm)   \\
\midrule
No Recon. & 15.7 & \textbf{48.5} & 80.5  \\
\midrule
Colorization & 63.9 & 47.0 & N/A  \\
Jigsaw Puzzle & 77.1 & 40.7 & N/A \\
%\midrule
Autoencoder & 65.6 & 42.9 & 51.1  \\
Inpainting & \textbf{88.3} & 46.5 & \textbf{46.6}  \\
\bottomrule[1.5pt]
\end{tabular}
\end{table}

\begin{table*}[h]
\centering
\vspace{-2pt}
\caption{\footnotesize{Performance of {\name} and reconstructive baselines on MPII for the downstream task of human pose estimation. $\uparrow$ indicates the larger the value, the better the performance. Note that the results here are for 2D pose estimation from images, whereas RF-based 3D pose estimation is in 3D, so the evaluation metrics are different.}}
\vspace{2pt}
\label{tab:result-pose}
\begin{threeparttable}
\resizebox{0.98\textwidth}{!}{
\begin{tabular}{c|c|c|c|c|c|c|c|c|c} 
\toprule[1.5pt]
\multicolumn{2}{c|}{\textsc{Metric}} & Head$^\uparrow$ & Shoulder$^\uparrow$ & Elbow$^\uparrow$ & Wrist$^\uparrow$ & Hip$^\uparrow$ & Knee$^\uparrow$ & Ankle$^\uparrow$ & PCKh$^\uparrow$ \\ 
\midrule
\midrule
\multirow{5}{*}{\begin{tabular}[c]{@{}c@{}}\textsc{Fixed}\\\textsc{feature}\\\textsc{extractor} \end{tabular}} 
%&Random init & 30.3 & 31.4 & 20.2 & 13.8 & 25.8 & 18.1 & 17.5 & 23.9 \\

%&SimCLR & 78.4 & 74.6 & 56.7 & 45.2 & 61.8 & 51.3 & 47.1 & 60.8 \\
%&MoCo & 79.2 & 75.1 & 57.4 & 45.9 & 62.4 & 52.0 & 47.6 & 61.4 \\

%&CPC & 78.0 & 74.3 & 56.0 & 44.8 & 61.2 & 51.4 & 46.5 & 60.3 \\
%&BYOL & 79.1 & 75.0 & 57.1 & 46.0 & 62.4 & 52.2 & 47.7 & 61.4 \\
&Inpainting  & 83.4 & 75.2 & 53.6 & 44.4 & 56.4 & 44.3 & 45.7 & 59.0  \\ 
&Colorization  & 79.5 & 71.2 & 49.6 & 42.1 & 54.2 & 40.7 & 41.9 & 55.1  \\ 
&Autoencoder  & 79.1 & 70.1 & 47.2 & 41.6 & 51.9 & 39.1 & 40.3 & 53.8  \\ 

%Recontruction   & 15.3  & 65.0 \\   
\cmidrule{2-10}
&\bf \name~(ours)                                                                                      & \bf 85.7 & \bf 78.8 & \bf 61.7 & \bf 51.3 & \bf 64.4 & \bf 55.6 & \bf 49.2 & \bf 65.1                                                                                            \\ 
&\bf \textsc{Improvements}                                                                                      
& \bf \textcolor{darkgreen}{\textbf{+2.3}}
& \bf \textcolor{darkgreen}{\textbf{+3.6}} 
& \bf \textcolor{darkgreen}{\textbf{+8.1}} 
& \bf \textcolor{darkgreen}{\textbf{+6.9}} 
& \bf \textcolor{darkgreen}{\textbf{+8.0}} 
& \bf \textcolor{darkgreen}{\textbf{+11.3}} 
& \bf \textcolor{darkgreen}{\textbf{+3.5}}
& \bf \textcolor{darkgreen}{\textbf{+6.1}}                                                                                          \\ 
%\hhline{=-==}
\midrule
\midrule
\multirow{5}{*}{\begin{tabular}[c]{@{}c@{}}\textsc{Fine-}\\\textsc{tuning} \end{tabular}} 
%& SimCLR & 96.2 & 94.7 & 87.3 & 81.2 & 87.5 & 81.0 & 77.2 & 87.1 \\
%& MoCo & 95.9 & 94.7 & 87.5 & 81.6 & 87.4 & 81.7 & 76.9 & 87.2 \\
%& CPC & 96.0 & 94.5 & 87.0 & 81.1 & 87.3 & 80.8 & 77.0 & 87.0 \\
%& BYOL & 96.2 & 94.8 & 87.5 & 81.4 & 87.6 & 81.5 & 77.0 & 87.2 \\
&Inpainting & 96.3 & \bf 95.2 & 87.9 & 82.1 & 87.8 & 82.5 & 77.6 & 87.7 \\ 
&Colorization & 96.2 & 95.1 & 87.7 & 82.1 & 87.8 & 82.5 & 77.5 & 87.6 \\ 
&Autoencoder & 96.0 & 94.9 & 87.6 & 82.0 & 87.6 & 82.4 & 77.3 & 87.5 \\ 

\cmidrule{2-10}
&\bf \name~(ours)                                                                                     & \bf 96.3 &94.9 & \bf 88.1 & \bf 82.3 & \bf 87.9 & \bf 82.8 & \bf 77.8 & \bf 87.8                                                                                                                                                                        \\
&\bf \textsc{Improvements}                                                                                      
& \bf \textcolor{darkgreen}{\textbf{+0.0}} 
& \bf \textcolor{lightblue}{\textbf{-0.3}}  
& \bf \textcolor{darkgreen}{\textbf{+0.2}} 
& \bf \textcolor{darkgreen}{\textbf{+0.2}}
& \bf \textcolor{darkgreen}{\textbf{+0.1}} 
& \bf \textcolor{darkgreen}{\textbf{+0.3}} 
& \bf \textcolor{darkgreen}{\textbf{+0.2}} 
& \bf \textcolor{darkgreen}{\textbf{+0.1}}                                                                                            \\ 

%\midrule
%\midrule
%\multicolumn{2}{c|}{\textsc{Supervised}}     & 96.3 & 95.1 & 87.9 & 82.2 & 87.8 & 82.7 & 77.8 & 87.7\\

\bottomrule[1.5pt]
\end{tabular}}
\end{threeparttable}
%\vspace{-15pt}
%\end{table*}
%
%
%\begin{table*}
\begin{tabular}{cc}
%\end{tabular}

\begin{minipage}{.52\linewidth}
\centering
\caption{\footnotesize{Performance on FairFace with {\name} and  different reconstructive unsupervised learning methods. The models are evaluated on downstream tasks of age, gender and ethnicity classification.}}
\label{tab:result-face}
\begin{threeparttable}
\resizebox{.98\textwidth}{!}{
\begin{tabular}{c|c|c|c|c} 
%\hline
\toprule[1.5pt]
\multicolumn{2}{c|}{\textsc{Metric}}                                                                                  & \begin{tabular}[c]{@{}c@{}}\textsc{Age cls} \\ \textsc{Acc.} (\%) \end{tabular} & \begin{tabular}[c]{@{}c@{}}\textsc{Gender cls} \\ \textsc{Acc.} (\%) \end{tabular} & \begin{tabular}[c]{@{}c@{}}\textsc{Ethn. cls} \\ \textsc{Acc.} (\%) \end{tabular} \\ 
\midrule\midrule
\multirow{6}{*}{\begin{tabular}[c]{@{}c@{}}\textsc{Fixed}\\\textsc{feature}\\\textsc{extractor} \end{tabular}} %&SimCLR                   & 43.9  & 78.1  & 61.7                                                                  \\
%&MoCo                      & 44.5  & 78.6  & 61.9                                                                  \\
%&CPC                                                                                                         & 43.5  & 76.2  & 61.0                                                                  \\ 
&Inpainting & 46.3  & 83.6  & 52.9  \\
&Colorization & 46.1  & 82.9  & 53.8  \\
&Autoencoder & 44.3  & 80.1  & 50.7  \\

%Recontruction   & 15.3  & 65.0 \\
%&Inpainting                                                                                                          & 15.3                                                                 & 65.0\\      
\cmidrule{2-5}
&\bf{\name~(ours)}  & \bf{50.0}  & \bf{87.2}  & \bf 61.2     \\ 
&\bf \textsc{Improvement}                                                                                      & \bf \textcolor{darkgreen}{\textbf{+3.7}}  & \textcolor{darkgreen}{\textbf{+3.6}}  & \textcolor{darkgreen}{\textbf{+7.4}} \\ 
%\hhline{=-==}
\midrule\midrule
\multirow{6}{*}{\begin{tabular}[c]{@{}c@{}}\textsc{Fine-}\\\textsc{tuning} \end{tabular}}
%& SimCLR  &54.3 & 91.1 & 69.1   \\
%& MoCo & 54.7 & 91.3 & 69.2  \\
%&CPC  & 54.2 & 91.0 & 68.8    \\ 
%&Inpainting                                                                                                          & 7.1                                                                   & 45.5                                                                  \\ 
%&BYOL & 54.6 &91.5 & \textbf{69.3} \\
&Inpainting & 55.0  & 91.8  & 68.3  \\
&Colorization & 54.9  & 92.0  & 68.6  \\
&Autoencoder & 54.5  & 91.3  & 67.9  \\
\cmidrule{2-5}
&\bf{\name~(ours)}                                                                                    &  \textbf{55.3}                                                                  &  \textbf{92.3}                 & \bf 69.0                                                 \\ 
&\bf \textsc{Improvement}                                                                                     & \bf \textcolor{darkgreen}{\textbf{+0.3}}      & \bf \textcolor{darkgreen}{\textbf{+0.3}}                                                         & \textcolor{darkgreen}{\textbf{+0.4}}                                                             \\ 
%\midrule\midrule
%\multicolumn{2}{c|}{\textsc{Supervised} on \textsc{Age}}                                                                      & 55.5 & 78.8  & 45.1                                                                 \\
%\multicolumn{2}{c|}{\textsc{Supervised} on \textsc{gender}}                                                                        & 43.3 & 92.5  & 45.4                                                                 \\
%\multicolumn{2}{c|}{\textsc{Supervised} on \textsc{Ethn.}}                                                                & 42.1 & 76.8  & 69.4                                                                \\
%\multicolumn{2}{c|}{\textsc{Supervised} on \textsc{All}}                                                                & 54.8 & 91.9  &  68.8                                                                \\
%\hline
\bottomrule[1.5pt]
\end{tabular}
}
\end{threeparttable}
\end{minipage}
&
\begin{minipage}{.44\linewidth}
\centering
%\vspace{7pt}
\caption{\footnotesize{Performance on Colorful-MNIST under different methods. The models are evaluated on the downstream tasks of digit classification and background object classification.}}
\label{tab:result-toy}
\begin{threeparttable}
\resizebox{0.98\textwidth}{!}{
\begin{tabular}{c|c|c|c} 
%\hline
\toprule[1.5pt]
\multicolumn{2}{c|}{\textsc{Metric}}                                                                                  & \begin{tabular}[c]{@{}c@{}}\textsc{Digit cls} \\ \textsc{Acc.} (\%) \end{tabular} & \begin{tabular}[c]{@{}c@{}}\textsc{Bkgd cls} \\ \textsc{Acc.} (\%) \end{tabular}  \\ 
\midrule\midrule
\multirow{6}{*}{\begin{tabular}[c]{@{}c@{}}\textsc{Fixed}\\\textsc{feature}\\\textsc{extractor} \end{tabular}} %&SimCLR                    & 14.9                                                                  & 47.3                                                                  \\
%&MoCo                                                                                                         & 15.7                                                                  & 48.5                                                                  \\
%&CPC                                                                                                          & 15.8                                                                  & 35.2                                                                  \\ 
%&BYOL & 15.5 & \textbf{49.0} \\
%Recontruction   & 15.3  & 65.0 \\
&Inpainting    & 84.7                  & 35.0\\     
&Colorization    & 80.7                  & 38.4\\      
&Autoencoder    & 81.0                  & 32.9\\      
 
\cmidrule{2-4}
&\bf{\name~(ours)}                                                                                      & \bf 88.3                                                                  & \bf 46.5                                                                  \\ 
&\bf \textsc{Improvement}                                                                                      & \bf \textcolor{darkgreen}{\textbf{+3.2}}                                                                & \textcolor{darkgreen}{\textbf{+8.1}} \\ 
%\hhline{=-==}
\midrule\midrule
\multirow{6}{*}{\begin{tabular}[c]{@{}c@{}}\textsc{Fine-}\\\textsc{tuning} \end{tabular}} 
%& SimCLR                               & 92.4                                                                   & 54.8                                                                  \\
%& MoCo                                                                                                         & 92.7                                                                   & 54.9                                                                  \\
%&CPC                                                                                                      & 92.3                                                                   & 54.7                                                                  \\ 
&Inpainting                                                                                                          & 92.9                                                                   & 54.5                                                                  \\ 
&Colorization & 92.5 & 54.5 \\
&Autoencoder & 92.4 & 54.1 \\

\cmidrule{2-4}
&\bf{\name~(ours)}                                                                                    & \bf 93.3                                                                   & \bf 54.7                                                                  \\ 
&\bf \textsc{Improvement}                                                                                     & \bf \textcolor{darkgreen}{\textbf{+0.4}}                                                               & \textcolor{darkgreen}{\textbf{+0.2}}                                                             \\ 
%\midrule\midrule
%\multicolumn{2}{c|}{\textsc{Supervised} on \textsc{digit}}                                                                      & 96.1                                                                   & 11.4                                                                  \\
%\multicolumn{2}{c|}{\textsc{Supervised} on \textsc{bkgd}}                                                                       & 12.9                                                                  & 56.7                                                                  \\
%\multicolumn{2}{c|}{\textsc{Supervised} on \textsc{digit} \&  \textsc{bkgd}}                                                                & 93.0                                                                   & 54.5                                                                  \\
%\hline
\bottomrule[1.5pt]
\end{tabular}
}
\end{threeparttable}

%\end{subtable}
%\hfill

%\begin{subtable}
\end{minipage}

\end{tabular}

%\vspace{-7pt}
%\end{table*}
%
%\begin{table*}[h]
\centering
\caption{\footnotesize{Evaluation of different models on different RF tasks under \textbf{fixed feature extractor} setting.
%where the RF feature encoder is initialized with pre-trained model using unsupervised learning methods, and the weights are frozen during downstream training. 
$\downarrow$ indicates the smaller the value, the better the performance; $\uparrow$ indicates the larger the value, the better the performance. Note that the '-' sign in 3D pose estimation improvements indicates better performance.}}
\label{tab:result-fixed}

\begin{threeparttable}
\resizebox{0.98\textwidth}{!}{
\begin{tabular}{l | c |c c|c c c|c c c}
%\hline
\toprule[1.5pt]
  Tasks & 3D Pose Estimation & \multicolumn{2}{c|}{Action Recognition} & \multicolumn{3}{c|}{Person Re-ID (Campus)} & \multicolumn{3}{c}{Person Re-ID (Home)} \\
\midrule
 \multirow{ 2}{*}{Metrics} &  \multirow{ 2}{*}{Pose \textsc{Err}.$^\downarrow$ (mm)} & \multicolumn{2}{c|}{mAP$^\uparrow$}  & \multirow{ 2}{*}{mAP$^\uparrow$} & \multirow{ 2}{*}{CMC-1$^\uparrow$} & \multirow{ 2}{*}{CMC-5$^\uparrow$} & \multirow{ 2}{*}{mAP$^\uparrow$} & \multirow{ 2}{*}{CMC-1$^\uparrow$} & \multirow{ 2}{*}{CMC-5$^\uparrow$} \\
 & & $\theta=0.1$ & $\theta=0.5$ & & & & & & \\
\midrule\midrule
Random init & 60.1 & 70.5  & 53.3 & 28.1 & 43.8 & 68.8 & 30.1 & 54.2 & 74.6 \\
\midrule
%SimCLR & 80.5 & 4.2 & 0 & 29.8 & 44.1 & 67.5 & 31.2 & 55.1 & 73.8 \\
%MoCo & 77.2 & 5.1 & 0.18 & 29.1 & 44.7 & 65.3 & 30.5 & 54.5 & 74.0 \\
%CPC & 78.7 & 3.6 & 0 & 30.0 & 42.7 & 69.5 & 30.7 & 54.0 & 75.3 \\
%BYOL & 79.3 & 4.7 & 0 & 29.5 & 44.4 & 66.7 & 30.7 & 54.6 & 73.5 \\
Inpainting & 51.1 & 72.3 & 65.5 & 49.8 & 73.1 & 90.5 & 38.5 & 64.2 & 84.7 \\
%Colorization & 51.1 & 72.3 & 65.5 & 49.8 & 73.1 & 90.5 & 38.5 & 64.2 & 84.7 \\
Autoencoder & 55.7 & 71.1 & 63.2 & 43.8 & 69.7 & 87.2 & 35.2 & 61.5 & 81.9 \\

\midrule
\textbf{\name(ours)} & \textbf{46.6} & \textbf{86.5} & \textbf{83.1} & \textbf{54.5} & \textbf{78.7} & \textbf{93.0} & \textbf{43.3} & \textbf{72.4} & \textbf{87.6}\\
\bf \textsc{Improvement} 
& \textcolor{darkgreen}{\textbf{-4.5}} 
 & \textcolor{darkgreen}{\textbf{+14.2}} 
 & \textcolor{darkgreen}{\textbf{+17.6}} 
 & \textcolor{darkgreen}{\textbf{+4.7}}  
 & \textcolor{darkgreen}{\textbf{+5.6}} 
 & \textcolor{darkgreen}{\textbf{+2.5}} 
 & \textcolor{darkgreen}{\textbf{+4.8}}
 & \textcolor{darkgreen}{\textbf{+8.2}} 
 & \textcolor{darkgreen}{\textbf{+2.9}}  
\\
%\midrule\midrule
%\textsc{Supervised \cite{li2019making,fan2020learning}} & 38.4 & 90.1  & 87.8 & 59.5 & 82.1 & 95.5 & 46.4 & 74.6 & 89.5 \\
%\hline 
\bottomrule[1.5pt]
\end{tabular}}
\end{threeparttable}
\vspace{-5pt}
%\end{table*}

%\begin{table*}[t]
\centering
\caption{\footnotesize{Evaluation of different models on different RF tasks under \textbf{fine-tuning} setting.
%where the RF feature encoder is initialized with pre-trained model using unsupervised learning methods, and then fine-tuned during downstream training. 
$\downarrow$ indicates the smaller the value, the better the performance; $\uparrow$ indicates the larger the value, the better the performance. Note that the '-' sign in 3D pose estimation improvements indicates better performance.}}
\label{tab:result-finetune}
\begin{threeparttable}
\resizebox{0.98\textwidth}{!}{
\begin{tabular}{l | c |c c|c c c|c c c}
%\hline
\toprule[1.5pt]
  Tasks & 3D Pose Estimation & \multicolumn{2}{c|}{Action Recognition} & \multicolumn{3}{c|}{Person Re-ID (Campus)} & \multicolumn{3}{c}{Person Re-ID (Home)} \\
\midrule
 \multirow{ 2}{*}{Metrics} &  \multirow{ 2}{*}{Pose \textsc{Err.}$^\downarrow$ (mm)} & \multicolumn{2}{c|}{mAP$^\uparrow$}  & \multirow{ 2}{*}{mAP$^\uparrow$} & \multirow{ 2}{*}{CMC-1$^\uparrow$} & \multirow{ 2}{*}{CMC-5$^\uparrow$} & \multirow{ 2}{*}{mAP$^\uparrow$} & \multirow{ 2}{*}{CMC-1$^\uparrow$} & \multirow{ 2}{*}{CMC-5$^\uparrow$} \\
 & & $\theta=0.1$ & $\theta=0.5$ & & & & & & \\
\midrule\midrule
Random init \cite{li2019making,fan2020learning} & 38.4 & 90.1  & 87.8 & 59.5 & 82.1 & 95.5 & 46.4 & 74.6 & 89.5 \\
\midrule
%SimCLR & 38.8 & 89.8 & 87.4 & 59.0 & 81.7 & 94.1 & 45.9 & 73.8 & 88.5 \\
%MoCo & 38.3 & 89.7 & 87.2 & 59.3 & 82.0 & 94.5 & 46.4 & 74.3 & 89.7 \\
%CPC & 38.6 & 89.9 & 87.5 & 59.4 & 81.5 & 94.0 & 46.0 & 74.5 & 89.1 \\
%BYOL & 38.5 & 89.7 & 87.2 & 59.4 & 81.9 & 94.5 & 46.6 & 74.5 & 89.5 \\
Inpainting & 36.2 &  91.7 & 88.7 & 60.1 & 83.3 & 95.5 & 47.5 & 75.3 & 90.3\\
Autoencoder & 36.9 &  91.2 & 87.9 & 59.7 & 82.8 & 94.9 & 46.8 & 74.7 & 89.9\\

\midrule
\textbf{\name (ours)} & \textbf{35.1} & \textbf{92.5} & \textbf{89.6} & \textbf{60.8} & \textbf{84.2} & \textbf{96.0} & \textbf{48.1} & \textbf{76.1} & \textbf{91.0}\\
\bf \textsc{Improvement} 
& \textcolor{darkgreen}{\textbf{-1.1}} 
 & \textcolor{darkgreen}{\textbf{+0.8}} 
 & \textcolor{darkgreen}{\textbf{+0.9}}  
 & \textcolor{darkgreen}{\textbf{+0.7}}  
 & \textcolor{darkgreen}{\textbf{+0.9}}  
 & \textcolor{darkgreen}{\textbf{+0.5}}  
 & \textcolor{darkgreen}{\textbf{+0.6}}  
 & \textcolor{darkgreen}{\textbf{+0.8}}  
 & \textcolor{darkgreen}{\textbf{+0.7}}  \\

\bottomrule[1.5pt]
\end{tabular}}
\end{threeparttable}
\vspace{-15pt}
\end{table*}

\textbf{Reconstructive Learning vs. \name}: In the main paper, we mainly compare \name~with contrastive learning since contrastive learning is the current unsupervised learning SOTA on ImageNet and outperforms reconstructive learning by a large margin \cite{chen2020simple,grill2020bootstrap}. Here, we also compare \name~with reconstructive learning on various datasets to demonstrate the effectiveness of the contrastive branch of \name. 
Tables [2-4]
%\ref{}
 compare {\name} with Inpainting \cite{pathak2016context}, Colorization \cite{zhang2016colorful} and Auto-encoder on the RGB datasets. As colorization is not applicable to RF inputs, we compare {\name} with Inpainting and Autoencoder on the RF datasets, as reported in Table \ref{tab:result-fixed} and Table \ref{tab:result-finetune}. The results demonstrate that \name~outperforms all reconstructive learning baselines by a large margin. This is because the contrastive branch in \name~can significantly improve the quality of the learned representation so it can achieve much better performance on downstream tasks.

\textbf{Masking as a Data Augmentation vs. \name}: In the reconstructive branch, \name~introduces masked input images or RF signals. Some may wonder whether the improvements are coming from this masking operation, since cutting out the input signals can be viewed as one way of augmentation \cite{chen2020simple}. However, here in Table \ref{tab:ablation-cutout}, we show the performance of MoCo with and without masking augmentation on Colorful-MNIST and RF-MMD (we use the same masking strategy as the reconstructive branch of \name). As shown in the table, the performance of MoCo stays similar with or without masking augmentation. This demonstrate that the improvements of \name~do not come from this augmentation.
\begin{table}[h]
\centering
\caption{Performance of MoCo on Colorful-MNIST and RF-MMD with and without masking augmentation (fixed feature encoder setting). The results demonstrate that simply adding masking as a data augmentation does not achieve similar improvements as \name.}
\label{tab:ablation-cutout}
\begin{tabular}{l |@{\hspace{0.2cm}} c|  c  @{\hspace{0.2cm}}  |c @{\hspace{0.2cm}}c  @{\hspace{0.2cm}}c}\toprule[1.5pt]
  & \multicolumn{2}{c|}{Colorful-MNIST} & RF-MMD  \\
\midrule
Recon. Tasks & \begin{tabular}[c]{@{}c@{}}\textsc{Digit cls} \\ \textsc{Acc.} (\%) \end{tabular} & \begin{tabular}[c]{@{}c@{}}\textsc{Bkgd cls} \\ \textsc{Acc.} (\%) \end{tabular}  &  Pose \textsc{Err}.$^\downarrow$ (mm)   & \\

\midrule
MoCo w/o masking & 15.7 & \textbf{48.5} & 77.2 \\
MoCo w/ masking & 15.2 & 48.4  & 78.0 \\
\name & \textbf{88.3} & 46.5 & \textbf{46.6} \\
\bottomrule[1.5pt]
\end{tabular}

\end{table}

\textbf{\name\ vs. Concatenation of Reconstructive and Contrastive Features}: Since \name~is a combination of reconstructive learning and contrastive learning, some may wonder whether similar improvements can be achieved by simply concatenating the features of the two unsupervised task, instead of the complementary role of the two tasks. However, in Table \ref{tab:ablation-multitask}, we show the performance of simply concatenating two encoder networks, one is trained only with reconstructive loss, and the other is trained only with contrastive loss (i.e., the encoder does not share parameters in Figure 2). As shown in the table, the performance of this setting is significantly worse than \name. This is because \name's improvement is because of the complementary role of contrastive learning and reconstructive learning. Without the regularization of reconstructive loss, the contrastive branch will be biased to shortcut. Without the contrastive loss, features supervised only by reconstructive loss will be lack of high-level information that can be used for downstream tasks. Therefore, the contrastive loss and reconstructive loss must operate on the same feature to complement each other. 

\begin{table}[h]
\centering
\caption{Performance of \name~and concatenation of reconstructive and contrastive features on Colorful-MNIST and RF-MMD (fixed feature encoder setting). The difference is whether the contrastive and reconstructive branch share the encoder parameters. The results demonstrate that simply concatenate the features from reconstructive and contrastive learning performs worse than \name.}
\label{tab:ablation-multitask}
\begin{tabular}{l |@{\hspace{0.2cm}} c| c @{\hspace{0.2cm}}|  c @{\hspace{0.2cm}}c  @{\hspace{0.2cm}}c}\toprule[1.5pt]
  & \multicolumn{2}{c|}{Colorful-MNIST} &  RF-MMD  \\
\midrule
Recon. Tasks &  \begin{tabular}[c]{@{}c@{}}\textsc{Digit cls} \\ \textsc{Acc.} (\%) \end{tabular} & \begin{tabular}[c]{@{}c@{}}\textsc{Bkgd cls} \\ \textsc{Acc.} (\%) \end{tabular}  & Pose \textsc{Err}.$^\downarrow$ (mm)  & \\

\midrule
Reconstructive $\oplus$ Contrastive& 84.5 & \textbf{48.4} & 50.9  \\
\name & \textbf{88.3} & 46.5& \textbf{46.6}  \\
\bottomrule[1.5pt]
\end{tabular}

\end{table}

\textbf{Benefits of Unlabeled Data for RF-Based Sensing}: By enabling RF-based tasks to leverage unsupervised representation learning, \name\ allows RF-based sensing to benefit from a large amount of unlabeled RF data. To evaluate the benefit of such unlabeled data,  we simulate the scenario where only a handful of labeled RF data is available and a large amount of RF data is unlabeled data. Specifically, we randomly select 10\% of the training set of RF-MMD to be RF-MMD-S to serves as the small labeled dataset. We compare the performance of \name~when it is pretrained on RF-MMD-S and RF-MMD and finetuned on RF-MMD-S. 

\begin{table}[h]
\centering
\caption{Performance of \name~on RF-MMD with a small amount of labeled data. The results in the table use for training 
RF-MMD-S, which is a randomly selected 10\% of RF-MMD for which the training uses the labels (fine-tuning setting). The the rest of the dataset is used without labels. The table shows that \name\ can further improve the performance with more unlabeled data.}
\label{tab:result-data}
\begin{tabular}{c |@{\hspace{0.2cm}} c c @{\hspace{0.2cm}} c @{\hspace{0.2cm}}c @{\hspace{0.2cm}}c}\toprule[1.5pt]
Methods & Pose \textsc{Err.}$^\downarrow$ (mm) \\
\midrule
Training from scratch (RF-MMD-S) & 48.7 \\
\name~on RF-MMD-S+finetune on RF-MMD-S & 45.0\\
\name~on RF-MMD+finetune on RF-MMD-S & 42.1\\
\bottomrule[1.5pt]
\end{tabular}

\end{table}

As shown in Table \ref{tab:result-data}, \name~can improve the performance of RF-based 3D pose estimation without using any additional unlabeled data. This is because \name~can learn a general representation of RF signals and thus provide better generalization ability. Indeed, \name\ improves the skeleton error by 2.9~mm by leveraging the unlabeled data. This demonstrates the potential of using \name\ to leverage large-scale unlabeled RF data to improve the performance of RF-based human sensing methods.

\textbf{Warm-up Training}: To show the effectiveness of the proposed warm-up training strategy (Sec. 3 (c)), we compare the results of warm-up training with the results of directly using the combined loss $\mathcal{L}$ (i.e., combining the reconstruction loss and the contrastive loss) from the beginning:
\begin{table}[h]
\centering
\caption{Performance of \name~on Colorful-MNIST and RF-MMD with and without warm-up training.}
\label{tab:result-warmup-rgb}
\begin{tabular}{l |@{\hspace{0.2cm}} c| c  @{\hspace{0.2cm}} | c @{\hspace{0.2cm}}c  @{\hspace{0.2cm}}c}\toprule[1.5pt]
  & \multicolumn{2}{c|}{Colorful-MNIST} &  RF-MMD  \\
\midrule
Warm-up Training  & \begin{tabular}[c]{@{}c@{}}\textsc{Digit cls} \\ \textsc{Acc.} (\%) \end{tabular} & \begin{tabular}[c]{@{}c@{}}\textsc{Bkgd cls} \\ \textsc{Acc.} (\%) \end{tabular}  & Pose \textsc{Err}.$^\downarrow$ (mm) &  \\
\midrule
No & 24.9 & \textbf{47.8} & 65.3  \\
Yes & \textbf{88.3} & 46.5 &\textbf{46.6}  \\
\bottomrule[1.5pt]
\end{tabular}

\end{table}

As shown in Table \ref{tab:result-warmup-rgb}, without the warm-up training, on Colorful-MNIST, \name~largely degenerates to become similar to the contrastive learning baselines and cannot learn good features related to digit classification, and on RF, \name~performs similar to just applying the contrastive loss without adding the reconstructive loss (46.6 mm skeleton error as reported in Table 3 of the paper). This indicates that without the warm-up phase, the contrastive loss can dominate the network causing it to learn the shortcut at the beginning, and that the network cannot later jump out of the local minimum associated with the shortcut. On the other hand, with warm-up training, the network first learns a coarse representation of the RF signals; then the contrastive loss helps the network learn more fine-grained representations.

\section*{Appendix B: Implementation Details}
In this section, we provide the implementation details of the models used in our experiments. All experiments are performed on 8 NVIDIA Titan X Pascal GPUs. On each dataset, we fix the batch size and training epochs for different baselines for a fair comparison. Other parameters for each baseline follow the original paper to optimize for its best performance. Code will also be released upon acceptance of the paper.

\textbf{ImageNet-100:} We use a standard ResNet-50 for the encoder network. The decoder network is a 11-layer deconvolutional network. The projection head for contrastive learning is a 2-layer non-linear head which embeds the feature into a 128-dimensional unit sphere. The same network structure is used for all baselines and \name. 

We follow the open repo of \cite{xiao2020should,grill2020bootstrap,chen2020simple} for the implementation of baselines and \name~on ImageNet-100. All baselines and \name~is trained for 500 epochs with a batch size of 256. For the reconstructive branch of \name, we mask out $3$ to $5$ rectangles at random locations in the image. The size of each square is chosen by setting its side randomly between 40 and 80 pixels. For the contrastive branch of \name, we apply the same training scheme as MoCo. The first 10 epochs are warm-up epochs, where we only train the network with the reconstruction loss $\mathcal{L}_r$. For later training, we set $\lambda_1=10$ and $\lambda=1$. For other RGB datasets, we mainly follows similar implementation as ImageNet-100.

\textbf{MPII:} We use the network structure similar to the one in \cite{xiao2018simple}. We use a ResNet-50 for the encoder network. Three deconvolutional layers with kernel size 4 and one convolutional layer with kernel size 1 is added on top of the encoded feature to transfer the feature into 13 heatmaps corresponding to 13 keypoints. For the contrastive branch, a 2-layer non-linear projection head is added on top of the encoded feature and embeds the feature into a 128-dimensional unit sphere. For the reconstructive branch, a decoder network similar to the pose estimation deconvolution network (only the number of output channels is changed to 3) is used to reconstruct the original image. Other implementation details are the same as ImageNet-100. 

For the baselines and \name, we train the network for 300 epochs with a batch size of  256. The data augmentation is the same as the baseline augmentations on ImageNet-100. 
For \name, the first 10 epochs are warm-up epochs, where we only train the network with the reconstruction loss $\mathcal{L}_r$.

\textbf{FairFace:} We use a standard ResNet-50 for the encoder network. The decoder network is a 11-layer deconvolutional network. The projection head for contrastive learning is a 2-layer non-linear head which embeds the feature into a 128-dimensional unit sphere. The same network structure is used for all baselines and \name. 

For the baselines and \name, we train the network for 1000 epochs with a batch size of  256. The data augmentation is the same as the baseline augmentations on ImageNet-100. 
For \name, the first 30 epochs are warm-up epochs, where we only train the network with the reconstruction loss $\mathcal{L}_r$.

\textbf{Colorful-MNIST:} We use a 6-layer ConvNet for the encoder. The encoder weights for the predictive and contrastive branches are shared. The decoder is a 6-layer deconvolutional network symmetric to the encoder. The projection head for contrastive learning is a 2-layer non-linear head which embeds the feature into a 64-dim normalized space. 

We use the SGD optimizer with 0.1 learning rate, 1e-4 weight decay, and 0.9 momentum to train the model for 200 epochs. The learning rate is scaled with a factor of 0.1 at epoch 150 and 175. The batch size is set to 512. The temperature for contrastive loss is set to 0.1. For \name, the first 30 epochs are warm-up epochs, where we only train the network with the reconstruction loss $\mathcal{L}_r$.

For \name, for each input image after augmentation with a size of $64$ by $64$ pixels, we randomly mask out $3$ to $5$ rectangle patches at random locations in the image and fill them with the average pixel value of the dataset. The size of each square is chosen by setting its side randomly between $10$ and $16$ pixels. 

\textbf{RF Experiments:} We use the same network architecture as prior works \cite{zhao2018rf,fan2020learning,li2019making}. Since there is no prior work that applies existing contrastive learning methods on RF data, we implement SimCLR \cite{chen2020simple}, MoCo \cite{he2020momentum}, CPC \cite{henaff2019data} and BYOL \cite{grill2020bootstrap} on RF data by ourselves as baselines. The SimCLR implementation is similar to the contrastive branch of \name~(Sec. 4.1). For MoCo, we use the same data augmentation operations as SimCLR, except the positive feature pairs are generated by two feature networks, a normal one and a momentum one. The loss is the same as the one used in \cite{he2020momentum}. For BYOL, we use the same data augmentation operations as SimCLR, and follow the implementation of \cite{grill2020bootstrap} to generate predictions, projections and loss. For CPC, we follow the design in \cite{henaff2019data}. Specifically, we add a GRU RNN after the RF feature extractor. The output of the GRU at every frame is then used as the context to predict the features in 1.5s in the future using the contrastive loss. 

For all the baseline contrastive approaches and \name, we train the network for 50 epochs with a batch size of 128, using the Adam optimizer with 1e-3 learning rate and 1e-5 weight decay. For the contrastive branch of \name, we follow SimCLR for simplicity, as we observe similar performance among different contrastive methods. The network is trained for 50 epochs. For \name~, the first 5 epochs as warm-up epochs trained with only the reconstruction loss. We set $\lambda_1=100$ and $\lambda=1$ since RF signals are typically sparse so $\lambda_1$ should be larger to balance the value of the two losses.

\section*{Appendix C: Experiments' Setup and Evaluation Metrics}

\noindent\textbf{Setup.} On ImageNet-100, as common in the literature, we evaluate the representations with the encoder fixed and only the linear classifier is trained. On all other datasets, we evaluate the representations under two different settings: fixed feature encoder setting and fine-tuning setting. In the fixed feature encoder setting, the ResNet encoder is fixed and only the classifier (FairFace, Colorful-MNIST), the 4-layer decoder network (MPII), or the task-specific head (RF Experiments) is trained; In the fine-tuning setting, the encoder is initialized with the pre-trained model and fine-tuned during training.

\noindent\textbf{Evaluation Metrics.}
For ImageNet-100, FairFace and Colorful-MNIST, the evaluation metrics are the standard Top-1 classification accuracy. For MPII, we evaluate the learned representations under the single pose estimation setting~\cite{andriluka20142d}. Each person is cropped using the approximate location and scale provided by the dataset. Similar to prior works, we report the PCKh (Percentage of Correct Keypoints that uses the matching threshold as 50\% of the head segment length) value of each keypoint and an overall weighted averaged PCKh over all keypoints (head, shoulder, elbow, wrist, hip, knee, ankle). 

For RF experiments, we use the performance metrics used by past work for each task. Specifically, for 3D pose estimation, we use the average $l_2$ distance between 14 predicted keypoints and their ground-truth locations as the evaluation metric. For action recognition, we use mean average precision (mAP) at different intersection-over-union (IoU) thresholds $\theta$ to evaluate the accuracy of the model in detecting and classifying an action event. For person re-identification, we separate the dataset into query set and gallery set. The query samples and gallery samples are then encoded to feature vectors. We calculate the cosine distance between the features of each query sample and each gallery sample, and rank the distance to get the top-N closest gallery samples for each query sample. Based on the ranking results, we compute the mean average precision (mAP) and the cumulative matching characteristic (CMC) at rank-1 and rank-5.
