# Supplementary material for: Unsupervised Learning for Human Sensing Using Radio Signals
Source: arXiv:2207.02370 source file (2022-07-06)
Supplement: Supplementary file 2 [file implementation.tex]

\section*{Appendix B: Implementation Details}
In this section, we provide the implementation details of the models used in our experiments. All experiments are performed on 8 NVIDIA Titan X Pascal GPUs. On each dataset, we fix the batch size and training epochs for different baselines for a fair comparison. Other parameters for each baseline follow the original paper to optimize for its best performance. Code will also be released upon acceptance of the paper.

\textbf{ImageNet-100:} We use a standard ResNet-50 for the encoder network. The decoder network is a 11-layer deconvolutional network. The projection head for contrastive learning is a 2-layer non-linear head which embeds the feature into a 128-dimensional unit sphere. The same network structure is used for all baselines and \name. 

We follow the open repo of \cite{xiao2020should,grill2020bootstrap,chen2020simple} for the implementation of baselines and \name~on ImageNet-100. All baselines and \name~is trained for 500 epochs with a batch size of 256. For the reconstructive branch of \name, we mask out $3$ to $5$ rectangles at random locations in the image. The size of each square is chosen by setting its side randomly between 40 and 80 pixels. For the contrastive branch of \name, we apply the same training scheme as MoCo. The first 10 epochs are warm-up epochs, where we only train the network with the reconstruction loss $\mathcal{L}_r$. For later training, we set $\lambda_1=10$ and $\lambda=1$. For other RGB datasets, we mainly follows similar implementation as ImageNet-100.

\textbf{MPII:} We use the network structure similar to the one in \cite{xiao2018simple}. We use a ResNet-50 for the encoder network. Three deconvolutional layers with kernel size 4 and one convolutional layer with kernel size 1 is added on top of the encoded feature to transfer the feature into 13 heatmaps corresponding to 13 keypoints. For the contrastive branch, a 2-layer non-linear projection head is added on top of the encoded feature and embeds the feature into a 128-dimensional unit sphere. For the reconstructive branch, a decoder network similar to the pose estimation deconvolution network (only the number of output channels is changed to 3) is used to reconstruct the original image. Other implementation details are the same as ImageNet-100. 

For the baselines and \name, we train the network for 300 epochs with a batch size of  256. The data augmentation is the same as the baseline augmentations on ImageNet-100. 
For \name, the first 10 epochs are warm-up epochs, where we only train the network with the reconstruction loss $\mathcal{L}_r$.

\textbf{FairFace:} We use a standard ResNet-50 for the encoder network. The decoder network is a 11-layer deconvolutional network. The projection head for contrastive learning is a 2-layer non-linear head which embeds the feature into a 128-dimensional unit sphere. The same network structure is used for all baselines and \name. 

For the baselines and \name, we train the network for 1000 epochs with a batch size of  256. The data augmentation is the same as the baseline augmentations on ImageNet-100. 
For \name, the first 30 epochs are warm-up epochs, where we only train the network with the reconstruction loss $\mathcal{L}_r$.

\textbf{Colorful-MNIST:} We use a 6-layer ConvNet for the encoder. The encoder weights for the predictive and contrastive branches are shared. The decoder is a 6-layer deconvolutional network symmetric to the encoder. The projection head for contrastive learning is a 2-layer non-linear head which embeds the feature into a 64-dim normalized space. 

We use the SGD optimizer with 0.1 learning rate, 1e-4 weight decay, and 0.9 momentum to train the model for 200 epochs. The learning rate is scaled with a factor of 0.1 at epoch 150 and 175. The batch size is set to 512. The temperature for contrastive loss is set to 0.1. For \name, the first 30 epochs are warm-up epochs, where we only train the network with the reconstruction loss $\mathcal{L}_r$.

For \name, for each input image after augmentation with a size of $64$ by $64$ pixels, we randomly mask out $3$ to $5$ rectangle patches at random locations in the image and fill them with the average pixel value of the dataset. The size of each square is chosen by setting its side randomly between $10$ and $16$ pixels. 

\textbf{RF Experiments:} We use the same network architecture as prior works \cite{zhao2018rf,fan2020learning,li2019making}. Since there is no prior work that applies existing contrastive learning methods on RF data, we implement SimCLR \cite{chen2020simple}, MoCo \cite{he2020momentum}, CPC \cite{henaff2019data} and BYOL \cite{grill2020bootstrap} on RF data by ourselves as baselines. The SimCLR implementation is similar to the contrastive branch of \name~(Sec. 4.1). For MoCo, we use the same data augmentation operations as SimCLR, except the positive feature pairs are generated by two feature networks, a normal one and a momentum one. The loss is the same as the one used in \cite{he2020momentum}. For BYOL, we use the same data augmentation operations as SimCLR, and follow the implementation of \cite{grill2020bootstrap} to generate predictions, projections and loss. For CPC, we follow the design in \cite{henaff2019data}. Specifically, we add a GRU RNN after the RF feature extractor. The output of the GRU at every frame is then used as the context to predict the features in 1.5s in the future using the contrastive loss. 

For all the baseline contrastive approaches and \name, we train the network for 50 epochs with a batch size of 128, using the Adam optimizer with 1e-3 learning rate and 1e-5 weight decay. For the contrastive branch of \name, we follow SimCLR for simplicity, as we observe similar performance among different contrastive methods. The network is trained for 50 epochs. For \name~, the first 5 epochs as warm-up epochs trained with only the reconstruction loss. We set $\lambda_1=100$ and $\lambda=1$ since RF signals are typically sparse so $\lambda_1$ should be larger to balance the value of the two losses.
