# Supplementary material for: Unsupervised Learning for Human Sensing Using Radio Signals
Source: arXiv:2207.02370 source file (2022-07-06)
Supplement: Supplementary file 3 [file results.tex]

\section*{Appendix A: Additional Results}
In this section, we provide additional results to better understand the good practices for applying \name~to RGB and RF data.

\textbf{Comparison of Different Reconstructive Tasks for \name's Reconstructive Branch}: In \name, we choose the inpainting task for the reconstructive branch. However, other reconstructive tasks can be potentially used for the reconstructive branch. In this section, we evaluate the performance of \name~with different reconstructive tasks including inpainting, auto-encoder, colorization \cite{zhang2016colorful}, and Jigsaw Puzzle \cite{noroozi2016unsupervised}. Table \ref{tab:ablation} shows \name's performance using different reconstructive task on Colorful-MNIST and RF-based 3D pose estimation (RF-MMD) under the fixed feature extractor setting. As shown in the table, all reconstructive tasks significantly reduce errors in comparison to using contrastive learning without any reconstruction task.  The table also shows that inpaintaing compares favorably to other tasks and works across modalities. Hence, we use inpainting as the default reconstructive task  in \name. 

\begin{table}[h]
\centering
\caption{Comparison of different reconstructive tasks for RCL's reconstructive branch. The table shows 
the performance of \name~on Colorful-MNIST and RF-MMD with different reconstructive tasks in its reconstructive branch for the fixed feature encoder setting. Colorization and Jigsaw Puzzle are not applicable to RF signals. Inpainting achieves the best performance and is applicability across modalities and tasks.}
\label{tab:ablation}
\begin{tabular}{l |@{\hspace{0.2cm}} c c @{\hspace{0.2cm}} |  c @{\hspace{0.2cm}}c  @{\hspace{0.2cm}}c}\toprule[1.5pt]

  & \multicolumn{2}{c|}{Colorful-MNIST}  &  RF-MMD \\
\midrule
Recon. Tasks & \begin{tabular}[c]{@{}c@{}}\textsc{Digit cls} \\ \textsc{Acc.} (\%) \end{tabular} & \begin{tabular}[c]{@{}c@{}}\textsc{Bkgd cls} \\ \textsc{Acc.} (\%) \end{tabular} & Pose \textsc{Err}.$^\downarrow$ (mm)   \\
\midrule
No Recon. & 15.7 & \textbf{48.5} & 80.5  \\
\midrule
Colorization & 63.9 & 47.0 & N/A  \\
Jigsaw Puzzle & 77.1 & 40.7 & N/A \\
%\midrule
Autoencoder & 65.6 & 42.9 & 51.1  \\
Inpainting & \textbf{88.3} & 46.5 & \textbf{46.6}  \\
\bottomrule[1.5pt]
\end{tabular}
\end{table}

\begin{table*}[h]
\centering
\vspace{-2pt}
\caption{\footnotesize{Performance of {\name} and reconstructive baselines on MPII for the downstream task of human pose estimation. $\uparrow$ indicates the larger the value, the better the performance. Note that the results here are for 2D pose estimation from images, whereas RF-based 3D pose estimation is in 3D, so the evaluation metrics are different.}}
\vspace{2pt}
\label{tab:result-pose}
\begin{threeparttable}
\resizebox{0.98\textwidth}{!}{
\begin{tabular}{c|c|c|c|c|c|c|c|c|c} 
\toprule[1.5pt]
\multicolumn{2}{c|}{\textsc{Metric}} & Head$^\uparrow$ & Shoulder$^\uparrow$ & Elbow$^\uparrow$ & Wrist$^\uparrow$ & Hip$^\uparrow$ & Knee$^\uparrow$ & Ankle$^\uparrow$ & PCKh$^\uparrow$ \\ 
\midrule
\midrule
\multirow{5}{*}{\begin{tabular}[c]{@{}c@{}}\textsc{Fixed}\\\textsc{feature}\\\textsc{extractor} \end{tabular}} 
%&Random init & 30.3 & 31.4 & 20.2 & 13.8 & 25.8 & 18.1 & 17.5 & 23.9 \\

%&SimCLR & 78.4 & 74.6 & 56.7 & 45.2 & 61.8 & 51.3 & 47.1 & 60.8 \\
%&MoCo & 79.2 & 75.1 & 57.4 & 45.9 & 62.4 & 52.0 & 47.6 & 61.4 \\

%&CPC & 78.0 & 74.3 & 56.0 & 44.8 & 61.2 & 51.4 & 46.5 & 60.3 \\
%&BYOL & 79.1 & 75.0 & 57.1 & 46.0 & 62.4 & 52.2 & 47.7 & 61.4 \\
&Inpainting  & 83.4 & 75.2 & 53.6 & 44.4 & 56.4 & 44.3 & 45.7 & 59.0  \\ 
&Colorization  & 79.5 & 71.2 & 49.6 & 42.1 & 54.2 & 40.7 & 41.9 & 55.1  \\ 
&Autoencoder  & 79.1 & 70.1 & 47.2 & 41.6 & 51.9 & 39.1 & 40.3 & 53.8  \\ 

%Recontruction   & 15.3  & 65.0 \\   
\cmidrule{2-10}
&\bf \name~(ours)                                                                                      & \bf 85.7 & \bf 78.8 & \bf 61.7 & \bf 51.3 & \bf 64.4 & \bf 55.6 & \bf 49.2 & \bf 65.1                                                                                            \\ 
&\bf \textsc{Improvements}                                                                                      
& \bf \textcolor{darkgreen}{\textbf{+2.3}}
& \bf \textcolor{darkgreen}{\textbf{+3.6}} 
& \bf \textcolor{darkgreen}{\textbf{+8.1}} 
& \bf \textcolor{darkgreen}{\textbf{+6.9}} 
& \bf \textcolor{darkgreen}{\textbf{+8.0}} 
& \bf \textcolor{darkgreen}{\textbf{+11.3}} 
& \bf \textcolor{darkgreen}{\textbf{+3.5}}
& \bf \textcolor{darkgreen}{\textbf{+6.1}}                                                                                          \\ 
%\hhline{=-==}
\midrule
\midrule
\multirow{5}{*}{\begin{tabular}[c]{@{}c@{}}\textsc{Fine-}\\\textsc{tuning} \end{tabular}} 
%& SimCLR & 96.2 & 94.7 & 87.3 & 81.2 & 87.5 & 81.0 & 77.2 & 87.1 \\
%& MoCo & 95.9 & 94.7 & 87.5 & 81.6 & 87.4 & 81.7 & 76.9 & 87.2 \\
%& CPC & 96.0 & 94.5 & 87.0 & 81.1 & 87.3 & 80.8 & 77.0 & 87.0 \\
%& BYOL & 96.2 & 94.8 & 87.5 & 81.4 & 87.6 & 81.5 & 77.0 & 87.2 \\
&Inpainting & 96.3 & \bf 95.2 & 87.9 & 82.1 & 87.8 & 82.5 & 77.6 & 87.7 \\ 
&Colorization & 96.2 & 95.1 & 87.7 & 82.1 & 87.8 & 82.5 & 77.5 & 87.6 \\ 
&Autoencoder & 96.0 & 94.9 & 87.6 & 82.0 & 87.6 & 82.4 & 77.3 & 87.5 \\ 

\cmidrule{2-10}
&\bf \name~(ours)                                                                                     & \bf 96.3 &94.9 & \bf 88.1 & \bf 82.3 & \bf 87.9 & \bf 82.8 & \bf 77.8 & \bf 87.8                                                                                                                                                                        \\
&\bf \textsc{Improvements}                                                                                      
& \bf \textcolor{darkgreen}{\textbf{+0.0}} 
& \bf \textcolor{lightblue}{\textbf{-0.3}}  
& \bf \textcolor{darkgreen}{\textbf{+0.2}} 
& \bf \textcolor{darkgreen}{\textbf{+0.2}}
& \bf \textcolor{darkgreen}{\textbf{+0.1}} 
& \bf \textcolor{darkgreen}{\textbf{+0.3}} 
& \bf \textcolor{darkgreen}{\textbf{+0.2}} 
& \bf \textcolor{darkgreen}{\textbf{+0.1}}                                                                                            \\ 

%\midrule
%\midrule
%\multicolumn{2}{c|}{\textsc{Supervised}}     & 96.3 & 95.1 & 87.9 & 82.2 & 87.8 & 82.7 & 77.8 & 87.7\\

\bottomrule[1.5pt]
\end{tabular}}
\end{threeparttable}
%\vspace{-15pt}
%\end{table*}
%
%
%\begin{table*}
\begin{tabular}{cc}
%\end{tabular}

\begin{minipage}{.52\linewidth}
\centering
\caption{\footnotesize{Performance on FairFace with {\name} and  different reconstructive unsupervised learning methods. The models are evaluated on downstream tasks of age, gender and ethnicity classification.}}
\label{tab:result-face}
\begin{threeparttable}
\resizebox{.98\textwidth}{!}{
\begin{tabular}{c|c|c|c|c} 
%\hline
\toprule[1.5pt]
\multicolumn{2}{c|}{\textsc{Metric}}                                                                                  & \begin{tabular}[c]{@{}c@{}}\textsc{Age cls} \\ \textsc{Acc.} (\%) \end{tabular} & \begin{tabular}[c]{@{}c@{}}\textsc{Gender cls} \\ \textsc{Acc.} (\%) \end{tabular} & \begin{tabular}[c]{@{}c@{}}\textsc{Ethn. cls} \\ \textsc{Acc.} (\%) \end{tabular} \\ 
\midrule\midrule
\multirow{6}{*}{\begin{tabular}[c]{@{}c@{}}\textsc{Fixed}\\\textsc{feature}\\\textsc{extractor} \end{tabular}} %&SimCLR                   & 43.9  & 78.1  & 61.7                                                                  \\
%&MoCo                      & 44.5  & 78.6  & 61.9                                                                  \\
%&CPC                                                                                                         & 43.5  & 76.2  & 61.0                                                                  \\ 
&Inpainting & 46.3  & 83.6  & 52.9  \\
&Colorization & 46.1  & 82.9  & 53.8  \\
&Autoencoder & 44.3  & 80.1  & 50.7  \\

%Recontruction   & 15.3  & 65.0 \\
%&Inpainting                                                                                                          & 15.3                                                                 & 65.0\\      
\cmidrule{2-5}
&\bf{\name~(ours)}  & \bf{50.0}  & \bf{87.2}  & \bf 61.2     \\ 
&\bf \textsc{Improvement}                                                                                      & \bf \textcolor{darkgreen}{\textbf{+3.7}}  & \textcolor{darkgreen}{\textbf{+3.6}}  & \textcolor{darkgreen}{\textbf{+7.4}} \\ 
%\hhline{=-==}
\midrule\midrule
\multirow{6}{*}{\begin{tabular}[c]{@{}c@{}}\textsc{Fine-}\\\textsc{tuning} \end{tabular}}
%& SimCLR  &54.3 & 91.1 & 69.1   \\
%& MoCo & 54.7 & 91.3 & 69.2  \\
%&CPC  & 54.2 & 91.0 & 68.8    \\ 
%&Inpainting                                                                                                          & 7.1                                                                   & 45.5                                                                  \\ 
%&BYOL & 54.6 &91.5 & \textbf{69.3} \\
&Inpainting & 55.0  & 91.8  & 68.3  \\
&Colorization & 54.9  & 92.0  & 68.6  \\
&Autoencoder & 54.5  & 91.3  & 67.9  \\
\cmidrule{2-5}
&\bf{\name~(ours)}                                                                                    &  \textbf{55.3}                                                                  &  \textbf{92.3}                 & \bf 69.0                                                 \\ 
&\bf \textsc{Improvement}                                                                                     & \bf \textcolor{darkgreen}{\textbf{+0.3}}      & \bf \textcolor{darkgreen}{\textbf{+0.3}}                                                         & \textcolor{darkgreen}{\textbf{+0.4}}                                                             \\ 
%\midrule\midrule
%\multicolumn{2}{c|}{\textsc{Supervised} on \textsc{Age}}                                                                      & 55.5 & 78.8  & 45.1                                                                 \\
%\multicolumn{2}{c|}{\textsc{Supervised} on \textsc{gender}}                                                                        & 43.3 & 92.5  & 45.4                                                                 \\
%\multicolumn{2}{c|}{\textsc{Supervised} on \textsc{Ethn.}}                                                                & 42.1 & 76.8  & 69.4                                                                \\
%\multicolumn{2}{c|}{\textsc{Supervised} on \textsc{All}}                                                                & 54.8 & 91.9  &  68.8                                                                \\
%\hline
\bottomrule[1.5pt]
\end{tabular}
}
\end{threeparttable}
\end{minipage}
&
\begin{minipage}{.44\linewidth}
\centering
%\vspace{7pt}
\caption{\footnotesize{Performance on Colorful-MNIST under different methods. The models are evaluated on the downstream tasks of digit classification and background object classification.}}
\label{tab:result-toy}
\begin{threeparttable}
\resizebox{0.98\textwidth}{!}{
\begin{tabular}{c|c|c|c} 
%\hline
\toprule[1.5pt]
\multicolumn{2}{c|}{\textsc{Metric}}                                                                                  & \begin{tabular}[c]{@{}c@{}}\textsc{Digit cls} \\ \textsc{Acc.} (\%) \end{tabular} & \begin{tabular}[c]{@{}c@{}}\textsc{Bkgd cls} \\ \textsc{Acc.} (\%) \end{tabular}  \\ 
\midrule\midrule
\multirow{6}{*}{\begin{tabular}[c]{@{}c@{}}\textsc{Fixed}\\\textsc{feature}\\\textsc{extractor} \end{tabular}} %&SimCLR                    & 14.9                                                                  & 47.3                                                                  \\
%&MoCo                                                                                                         & 15.7                                                                  & 48.5                                                                  \\
%&CPC                                                                                                          & 15.8                                                                  & 35.2                                                                  \\ 
%&BYOL & 15.5 & \textbf{49.0} \\
%Recontruction   & 15.3  & 65.0 \\
&Inpainting    & 84.7                  & 35.0\\     
&Colorization    & 80.7                  & 38.4\\      
&Autoencoder    & 81.0                  & 32.9\\      
 
\cmidrule{2-4}
&\bf{\name~(ours)}                                                                                      & \bf 88.3                                                                  & \bf 46.5                                                                  \\ 
&\bf \textsc{Improvement}                                                                                      & \bf \textcolor{darkgreen}{\textbf{+3.2}}                                                                & \textcolor{darkgreen}{\textbf{+8.1}} \\ 
%\hhline{=-==}
\midrule\midrule
\multirow{6}{*}{\begin{tabular}[c]{@{}c@{}}\textsc{Fine-}\\\textsc{tuning} \end{tabular}} 
%& SimCLR                               & 92.4                                                                   & 54.8                                                                  \\
%& MoCo                                                                                                         & 92.7                                                                   & 54.9                                                                  \\
%&CPC                                                                                                      & 92.3                                                                   & 54.7                                                                  \\ 
&Inpainting                                                                                                          & 92.9                                                                   & 54.5                                                                  \\ 
&Colorization & 92.5 & 54.5 \\
&Autoencoder & 92.4 & 54.1 \\

\cmidrule{2-4}
&\bf{\name~(ours)}                                                                                    & \bf 93.3                                                                   & \bf 54.7                                                                  \\ 
&\bf \textsc{Improvement}                                                                                     & \bf \textcolor{darkgreen}{\textbf{+0.4}}                                                               & \textcolor{darkgreen}{\textbf{+0.2}}                                                             \\ 
%\midrule\midrule
%\multicolumn{2}{c|}{\textsc{Supervised} on \textsc{digit}}                                                                      & 96.1                                                                   & 11.4                                                                  \\
%\multicolumn{2}{c|}{\textsc{Supervised} on \textsc{bkgd}}                                                                       & 12.9                                                                  & 56.7                                                                  \\
%\multicolumn{2}{c|}{\textsc{Supervised} on \textsc{digit} \&  \textsc{bkgd}}                                                                & 93.0                                                                   & 54.5                                                                  \\
%\hline
\bottomrule[1.5pt]
\end{tabular}
}
\end{threeparttable}

%\end{subtable}
%\hfill

%\begin{subtable}
\end{minipage}

\end{tabular}

%\vspace{-7pt}
%\end{table*}
%
%\begin{table*}[h]
\centering
\caption{\footnotesize{Evaluation of different models on different RF tasks under \textbf{fixed feature extractor} setting.
%where the RF feature encoder is initialized with pre-trained model using unsupervised learning methods, and the weights are frozen during downstream training. 
$\downarrow$ indicates the smaller the value, the better the performance; $\uparrow$ indicates the larger the value, the better the performance. Note that the '-' sign in 3D pose estimation improvements indicates better performance.}}
\label{tab:result-fixed}

\begin{threeparttable}
\resizebox{0.98\textwidth}{!}{
\begin{tabular}{l | c |c c|c c c|c c c}
%\hline
\toprule[1.5pt]
  Tasks & 3D Pose Estimation & \multicolumn{2}{c|}{Action Recognition} & \multicolumn{3}{c|}{Person Re-ID (Campus)} & \multicolumn{3}{c}{Person Re-ID (Home)} \\
\midrule
 \multirow{ 2}{*}{Metrics} &  \multirow{ 2}{*}{Pose \textsc{Err}.$^\downarrow$ (mm)} & \multicolumn{2}{c|}{mAP$^\uparrow$}  & \multirow{ 2}{*}{mAP$^\uparrow$} & \multirow{ 2}{*}{CMC-1$^\uparrow$} & \multirow{ 2}{*}{CMC-5$^\uparrow$} & \multirow{ 2}{*}{mAP$^\uparrow$} & \multirow{ 2}{*}{CMC-1$^\uparrow$} & \multirow{ 2}{*}{CMC-5$^\uparrow$} \\
 & & $\theta=0.1$ & $\theta=0.5$ & & & & & & \\
\midrule\midrule
Random init & 60.1 & 70.5  & 53.3 & 28.1 & 43.8 & 68.8 & 30.1 & 54.2 & 74.6 \\
\midrule
%SimCLR & 80.5 & 4.2 & 0 & 29.8 & 44.1 & 67.5 & 31.2 & 55.1 & 73.8 \\
%MoCo & 77.2 & 5.1 & 0.18 & 29.1 & 44.7 & 65.3 & 30.5 & 54.5 & 74.0 \\
%CPC & 78.7 & 3.6 & 0 & 30.0 & 42.7 & 69.5 & 30.7 & 54.0 & 75.3 \\
%BYOL & 79.3 & 4.7 & 0 & 29.5 & 44.4 & 66.7 & 30.7 & 54.6 & 73.5 \\
Inpainting & 51.1 & 72.3 & 65.5 & 49.8 & 73.1 & 90.5 & 38.5 & 64.2 & 84.7 \\
%Colorization & 51.1 & 72.3 & 65.5 & 49.8 & 73.1 & 90.5 & 38.5 & 64.2 & 84.7 \\
Autoencoder & 55.7 & 71.1 & 63.2 & 43.8 & 69.7 & 87.2 & 35.2 & 61.5 & 81.9 \\

\midrule
\textbf{\name(ours)} & \textbf{46.6} & \textbf{86.5} & \textbf{83.1} & \textbf{54.5} & \textbf{78.7} & \textbf{93.0} & \textbf{43.3} & \textbf{72.4} & \textbf{87.6}\\
\bf \textsc{Improvement} 
& \textcolor{darkgreen}{\textbf{-4.5}} 
 & \textcolor{darkgreen}{\textbf{+14.2}} 
 & \textcolor{darkgreen}{\textbf{+17.6}} 
 & \textcolor{darkgreen}{\textbf{+4.7}}  
 & \textcolor{darkgreen}{\textbf{+5.6}} 
 & \textcolor{darkgreen}{\textbf{+2.5}} 
 & \textcolor{darkgreen}{\textbf{+4.8}}
 & \textcolor{darkgreen}{\textbf{+8.2}} 
 & \textcolor{darkgreen}{\textbf{+2.9}}  
\\
%\midrule\midrule
%\textsc{Supervised \cite{li2019making,fan2020learning}} & 38.4 & 90.1  & 87.8 & 59.5 & 82.1 & 95.5 & 46.4 & 74.6 & 89.5 \\
%\hline 
\bottomrule[1.5pt]
\end{tabular}}
\end{threeparttable}
\vspace{-5pt}
%\end{table*}

%\begin{table*}[t]
\centering
\caption{\footnotesize{Evaluation of different models on different RF tasks under \textbf{fine-tuning} setting.
%where the RF feature encoder is initialized with pre-trained model using unsupervised learning methods, and then fine-tuned during downstream training. 
$\downarrow$ indicates the smaller the value, the better the performance; $\uparrow$ indicates the larger the value, the better the performance. Note that the '-' sign in 3D pose estimation improvements indicates better performance.}}
\label{tab:result-finetune}
\begin{threeparttable}
\resizebox{0.98\textwidth}{!}{
\begin{tabular}{l | c |c c|c c c|c c c}
%\hline
\toprule[1.5pt]
  Tasks & 3D Pose Estimation & \multicolumn{2}{c|}{Action Recognition} & \multicolumn{3}{c|}{Person Re-ID (Campus)} & \multicolumn{3}{c}{Person Re-ID (Home)} \\
\midrule
 \multirow{ 2}{*}{Metrics} &  \multirow{ 2}{*}{Pose \textsc{Err.}$^\downarrow$ (mm)} & \multicolumn{2}{c|}{mAP$^\uparrow$}  & \multirow{ 2}{*}{mAP$^\uparrow$} & \multirow{ 2}{*}{CMC-1$^\uparrow$} & \multirow{ 2}{*}{CMC-5$^\uparrow$} & \multirow{ 2}{*}{mAP$^\uparrow$} & \multirow{ 2}{*}{CMC-1$^\uparrow$} & \multirow{ 2}{*}{CMC-5$^\uparrow$} \\
 & & $\theta=0.1$ & $\theta=0.5$ & & & & & & \\
\midrule\midrule
Random init \cite{li2019making,fan2020learning} & 38.4 & 90.1  & 87.8 & 59.5 & 82.1 & 95.5 & 46.4 & 74.6 & 89.5 \\
\midrule
%SimCLR & 38.8 & 89.8 & 87.4 & 59.0 & 81.7 & 94.1 & 45.9 & 73.8 & 88.5 \\
%MoCo & 38.3 & 89.7 & 87.2 & 59.3 & 82.0 & 94.5 & 46.4 & 74.3 & 89.7 \\
%CPC & 38.6 & 89.9 & 87.5 & 59.4 & 81.5 & 94.0 & 46.0 & 74.5 & 89.1 \\
%BYOL & 38.5 & 89.7 & 87.2 & 59.4 & 81.9 & 94.5 & 46.6 & 74.5 & 89.5 \\
Inpainting & 36.2 &  91.7 & 88.7 & 60.1 & 83.3 & 95.5 & 47.5 & 75.3 & 90.3\\
Autoencoder & 36.9 &  91.2 & 87.9 & 59.7 & 82.8 & 94.9 & 46.8 & 74.7 & 89.9\\

\midrule
\textbf{\name (ours)} & \textbf{35.1} & \textbf{92.5} & \textbf{89.6} & \textbf{60.8} & \textbf{84.2} & \textbf{96.0} & \textbf{48.1} & \textbf{76.1} & \textbf{91.0}\\
\bf \textsc{Improvement} 
& \textcolor{darkgreen}{\textbf{-1.1}} 
 & \textcolor{darkgreen}{\textbf{+0.8}} 
 & \textcolor{darkgreen}{\textbf{+0.9}}  
 & \textcolor{darkgreen}{\textbf{+0.7}}  
 & \textcolor{darkgreen}{\textbf{+0.9}}  
 & \textcolor{darkgreen}{\textbf{+0.5}}  
 & \textcolor{darkgreen}{\textbf{+0.6}}  
 & \textcolor{darkgreen}{\textbf{+0.8}}  
 & \textcolor{darkgreen}{\textbf{+0.7}}  \\

\bottomrule[1.5pt]
\end{tabular}}
\end{threeparttable}
\vspace{-15pt}
\end{table*}

\textbf{Reconstructive Learning vs. \name}: In the main paper, we mainly compare \name~with contrastive learning since contrastive learning is the current unsupervised learning SOTA on ImageNet and outperforms reconstructive learning by a large margin \cite{chen2020simple,grill2020bootstrap}. Here, we also compare \name~with reconstructive learning on various datasets to demonstrate the effectiveness of the contrastive branch of \name. 
Tables [2-4]
%\ref{}
 compare {\name} with Inpainting \cite{pathak2016context}, Colorization \cite{zhang2016colorful} and Auto-encoder on the RGB datasets. As colorization is not applicable to RF inputs, we compare {\name} with Inpainting and Autoencoder on the RF datasets, as reported in Table \ref{tab:result-fixed} and Table \ref{tab:result-finetune}. The results demonstrate that \name~outperforms all reconstructive learning baselines by a large margin. This is because the contrastive branch in \name~can significantly improve the quality of the learned representation so it can achieve much better performance on downstream tasks.

\textbf{Masking as a Data Augmentation vs. \name}: In the reconstructive branch, \name~introduces masked input images or RF signals. Some may wonder whether the improvements are coming from this masking operation, since cutting out the input signals can be viewed as one way of augmentation \cite{chen2020simple}. However, here in Table \ref{tab:ablation-cutout}, we show the performance of MoCo with and without masking augmentation on Colorful-MNIST and RF-MMD (we use the same masking strategy as the reconstructive branch of \name). As shown in the table, the performance of MoCo stays similar with or without masking augmentation. This demonstrate that the improvements of \name~do not come from this augmentation.
\begin{table}[h]
\centering
\caption{Performance of MoCo on Colorful-MNIST and RF-MMD with and without masking augmentation (fixed feature encoder setting). The results demonstrate that simply adding masking as a data augmentation does not achieve similar improvements as \name.}
\label{tab:ablation-cutout}
\begin{tabular}{l |@{\hspace{0.2cm}} c|  c  @{\hspace{0.2cm}}  |c @{\hspace{0.2cm}}c  @{\hspace{0.2cm}}c}\toprule[1.5pt]
  & \multicolumn{2}{c|}{Colorful-MNIST} & RF-MMD  \\
\midrule
Recon. Tasks & \begin{tabular}[c]{@{}c@{}}\textsc{Digit cls} \\ \textsc{Acc.} (\%) \end{tabular} & \begin{tabular}[c]{@{}c@{}}\textsc{Bkgd cls} \\ \textsc{Acc.} (\%) \end{tabular}  &  Pose \textsc{Err}.$^\downarrow$ (mm)   & \\

\midrule
MoCo w/o masking & 15.7 & \textbf{48.5} & 77.2 \\
MoCo w/ masking & 15.2 & 48.4  & 78.0 \\
\name & \textbf{88.3} & 46.5 & \textbf{46.6} \\
\bottomrule[1.5pt]
\end{tabular}

\end{table}

\textbf{\name\ vs. Concatenation of Reconstructive and Contrastive Features}: Since \name~is a combination of reconstructive learning and contrastive learning, some may wonder whether similar improvements can be achieved by simply concatenating the features of the two unsupervised task, instead of the complementary role of the two tasks. However, in Table \ref{tab:ablation-multitask}, we show the performance of simply concatenating two encoder networks, one is trained only with reconstructive loss, and the other is trained only with contrastive loss (i.e., the encoder does not share parameters in Figure 2). As shown in the table, the performance of this setting is significantly worse than \name. This is because \name's improvement is because of the complementary role of contrastive learning and reconstructive learning. Without the regularization of reconstructive loss, the contrastive branch will be biased to shortcut. Without the contrastive loss, features supervised only by reconstructive loss will be lack of high-level information that can be used for downstream tasks. Therefore, the contrastive loss and reconstructive loss must operate on the same feature to complement each other. 

\begin{table}[h]
\centering
\caption{Performance of \name~and concatenation of reconstructive and contrastive features on Colorful-MNIST and RF-MMD (fixed feature encoder setting). The difference is whether the contrastive and reconstructive branch share the encoder parameters. The results demonstrate that simply concatenate the features from reconstructive and contrastive learning performs worse than \name.}
\label{tab:ablation-multitask}
\begin{tabular}{l |@{\hspace{0.2cm}} c| c @{\hspace{0.2cm}}|  c @{\hspace{0.2cm}}c  @{\hspace{0.2cm}}c}\toprule[1.5pt]
  & \multicolumn{2}{c|}{Colorful-MNIST} &  RF-MMD  \\
\midrule
Recon. Tasks &  \begin{tabular}[c]{@{}c@{}}\textsc{Digit cls} \\ \textsc{Acc.} (\%) \end{tabular} & \begin{tabular}[c]{@{}c@{}}\textsc{Bkgd cls} \\ \textsc{Acc.} (\%) \end{tabular}  & Pose \textsc{Err}.$^\downarrow$ (mm)  & \\

\midrule
Reconstructive $\oplus$ Contrastive& 84.5 & \textbf{48.4} & 50.9  \\
\name & \textbf{88.3} & 46.5& \textbf{46.6}  \\
\bottomrule[1.5pt]
\end{tabular}

\end{table}

\textbf{Benefits of Unlabeled Data for RF-Based Sensing}: By enabling RF-based tasks to leverage unsupervised representation learning, \name\ allows RF-based sensing to benefit from a large amount of unlabeled RF data. To evaluate the benefit of such unlabeled data,  we simulate the scenario where only a handful of labeled RF data is available and a large amount of RF data is unlabeled data. Specifically, we randomly select 10\% of the training set of RF-MMD to be RF-MMD-S to serves as the small labeled dataset. We compare the performance of \name~when it is pretrained on RF-MMD-S and RF-MMD and finetuned on RF-MMD-S. 

\begin{table}[h]
\centering
\caption{Performance of \name~on RF-MMD with a small amount of labeled data. The results in the table use for training 
RF-MMD-S, which is a randomly selected 10\% of RF-MMD for which the training uses the labels (fine-tuning setting). The the rest of the dataset is used without labels. The table shows that \name\ can further improve the performance with more unlabeled data.}
\label{tab:result-data}
\begin{tabular}{c |@{\hspace{0.2cm}} c c @{\hspace{0.2cm}} c @{\hspace{0.2cm}}c @{\hspace{0.2cm}}c}\toprule[1.5pt]
Methods & Pose \textsc{Err.}$^\downarrow$ (mm) \\
\midrule
Training from scratch (RF-MMD-S) & 48.7 \\
\name~on RF-MMD-S+finetune on RF-MMD-S & 45.0\\
\name~on RF-MMD+finetune on RF-MMD-S & 42.1\\
\bottomrule[1.5pt]
\end{tabular}

\end{table}

As shown in Table \ref{tab:result-data}, \name~can improve the performance of RF-based 3D pose estimation without using any additional unlabeled data. This is because \name~can learn a general representation of RF signals and thus provide better generalization ability. Indeed, \name\ improves the skeleton error by 2.9~mm by leveraging the unlabeled data. This demonstrates the potential of using \name\ to leverage large-scale unlabeled RF data to improve the performance of RF-based human sensing methods.

\textbf{Warm-up Training}: To show the effectiveness of the proposed warm-up training strategy (Sec. 3 (c)), we compare the results of warm-up training with the results of directly using the combined loss $\mathcal{L}$ (i.e., combining the reconstruction loss and the contrastive loss) from the beginning:
\begin{table}[h]
\centering
\caption{Performance of \name~on Colorful-MNIST and RF-MMD with and without warm-up training.}
\label{tab:result-warmup-rgb}
\begin{tabular}{l |@{\hspace{0.2cm}} c| c  @{\hspace{0.2cm}} | c @{\hspace{0.2cm}}c  @{\hspace{0.2cm}}c}\toprule[1.5pt]
  & \multicolumn{2}{c|}{Colorful-MNIST} &  RF-MMD  \\
\midrule
Warm-up Training  & \begin{tabular}[c]{@{}c@{}}\textsc{Digit cls} \\ \textsc{Acc.} (\%) \end{tabular} & \begin{tabular}[c]{@{}c@{}}\textsc{Bkgd cls} \\ \textsc{Acc.} (\%) \end{tabular}  & Pose \textsc{Err}.$^\downarrow$ (mm) &  \\
\midrule
No & 24.9 & \textbf{47.8} & 65.3  \\
Yes & \textbf{88.3} & 46.5 &\textbf{46.6}  \\
\bottomrule[1.5pt]
\end{tabular}

\end{table}

As shown in Table \ref{tab:result-warmup-rgb}, without the warm-up training, on Colorful-MNIST, \name~largely degenerates to become similar to the contrastive learning baselines and cannot learn good features related to digit classification, and on RF, \name~performs similar to just applying the contrastive loss without adding the reconstructive loss (46.6 mm skeleton error as reported in Table 3 of the paper). This indicates that without the warm-up phase, the contrastive loss can dominate the network causing it to learn the shortcut at the beginning, and that the network cannot later jump out of the local minimum associated with the shortcut. On the other hand, with warm-up training, the network first learns a coarse representation of the RF signals; then the contrastive loss helps the network learn more fine-grained representations.
