# Supplementary material for: Unsupervised Learning for Human Sensing Using Radio Signals
Source: arXiv:2207.02370 source file (2022-07-06)
Supplement: Supplementary file 4 [file setup.tex]

\section*{Appendix C: Experiments' Setup and Evaluation Metrics}

\noindent\textbf{Setup.} On ImageNet-100, as common in the literature, we evaluate the representations with the encoder fixed and only the linear classifier is trained. On all other datasets, we evaluate the representations under two different settings: fixed feature encoder setting and fine-tuning setting. In the fixed feature encoder setting, the ResNet encoder is fixed and only the classifier (FairFace, Colorful-MNIST), the 4-layer decoder network (MPII), or the task-specific head (RF Experiments) is trained; In the fine-tuning setting, the encoder is initialized with the pre-trained model and fine-tuned during training.

\noindent\textbf{Evaluation Metrics.}
For ImageNet-100, FairFace and Colorful-MNIST, the evaluation metrics are the standard Top-1 classification accuracy. For MPII, we evaluate the learned representations under the single pose estimation setting~\cite{andriluka20142d}. Each person is cropped using the approximate location and scale provided by the dataset. Similar to prior works, we report the PCKh (Percentage of Correct Keypoints that uses the matching threshold as 50\% of the head segment length) value of each keypoint and an overall weighted averaged PCKh over all keypoints (head, shoulder, elbow, wrist, hip, knee, ankle). 

For RF experiments, we use the performance metrics used by past work for each task. Specifically, for 3D pose estimation, we use the average $l_2$ distance between 14 predicted keypoints and their ground-truth locations as the evaluation metric. For action recognition, we use mean average precision (mAP) at different intersection-over-union (IoU) thresholds $\theta$ to evaluate the accuracy of the model in detecting and classifying an action event. For person re-identification, we separate the dataset into query set and gallery set. The query samples and gallery samples are then encoded to feature vectors. We calculate the cosine distance between the features of each query sample and each gallery sample, and rank the distance to get the top-N closest gallery samples for each query sample. Based on the ranking results, we compute the mean average precision (mAP) and the cumulative matching characteristic (CMC) at rank-1 and rank-5.
